# Supplementary material for: Program Synthesis with Pragmatic Communication
Source: arXiv:2007.05060 source file (2020-10-21)
Supplement: Supplementary file 1 [file suppliment.tex]

\section{Suppliment}
I am Suppliment
